# Supplementary material for: Sketch2Stress: Sketching with Structural Stress Awareness
Source: arXiv:2306.05911 source file (2023-12-11)
Supplement: Supplementary file 1 [file supplemental_content.tex]

\begin{figure}[htb]
    \centering
    \includegraphics[width=1\linewidth]{figs/supplemental_network_im.pdf}
    \caption{\label{fig:fig_supple_sketch_im_network}
            Network structure of the sketch implicit model.}
\end{figure}

\begin{figure}[htb]
    \centering
    \includegraphics[width=1\linewidth]{figs/supplemental_network_assembly.pdf}
    \caption{\label{fig:fig_supple_sketch_assembly_network}
            Spatial transformation network (STN) for sketch assembly.}
\end{figure}

\begin{figure*}[htb]
    \centering
    \includegraphics[width=0.98\linewidth]{figs/fig_supplemental_fig1_v2.pdf}
    \caption{\label{fig:fig_supple_more_results1}
           Visual results of our method. Each triplet contains an input sketch (Left), the sketch after part beautification (Middle), and the final result after structure beautification (Right). Please zoom in for better visualization.}
\end{figure*}

\begin{figure*}[htb]
    \centering
    \includegraphics[width=0.98\linewidth]{figs/fig_supplemental_fig2_v2.pdf}
    \caption{\label{fig:fig_supple_more_results1}
        Visual results of our method. Each triplet contains an input sketch (Left), the sketch after part beautification (Middle), and the final result after structure beautification (Right). Please zoom in for better visualization. }
\end{figure*}

\begin{figure*}[tb]
    \centering
    \includegraphics[width=0.98\linewidth]{figs/fig_supplemental_fig3_v3.pdf}
    \caption{\label{fig:fig_supple_more_results1}
        Visual results of our method. Each triplet contains an input sketch (Left), the sketch after part beautification (Middle), and the final result after structure beautification (Right). Please zoom in for better visualization.}
\end{figure*}
