# Supplementary material for: Sketch2Stress: Sketching with Structural Stress Awareness
Source: arXiv:2306.05911 source file (2023-12-11)
Supplement: Supplementary file 4 [file fig_supplemental_qualititive.tex]

\begin{figure*}[t]{
    \centering
    % \vspace{-5mm}
    \includegraphics[width=\linewidth]{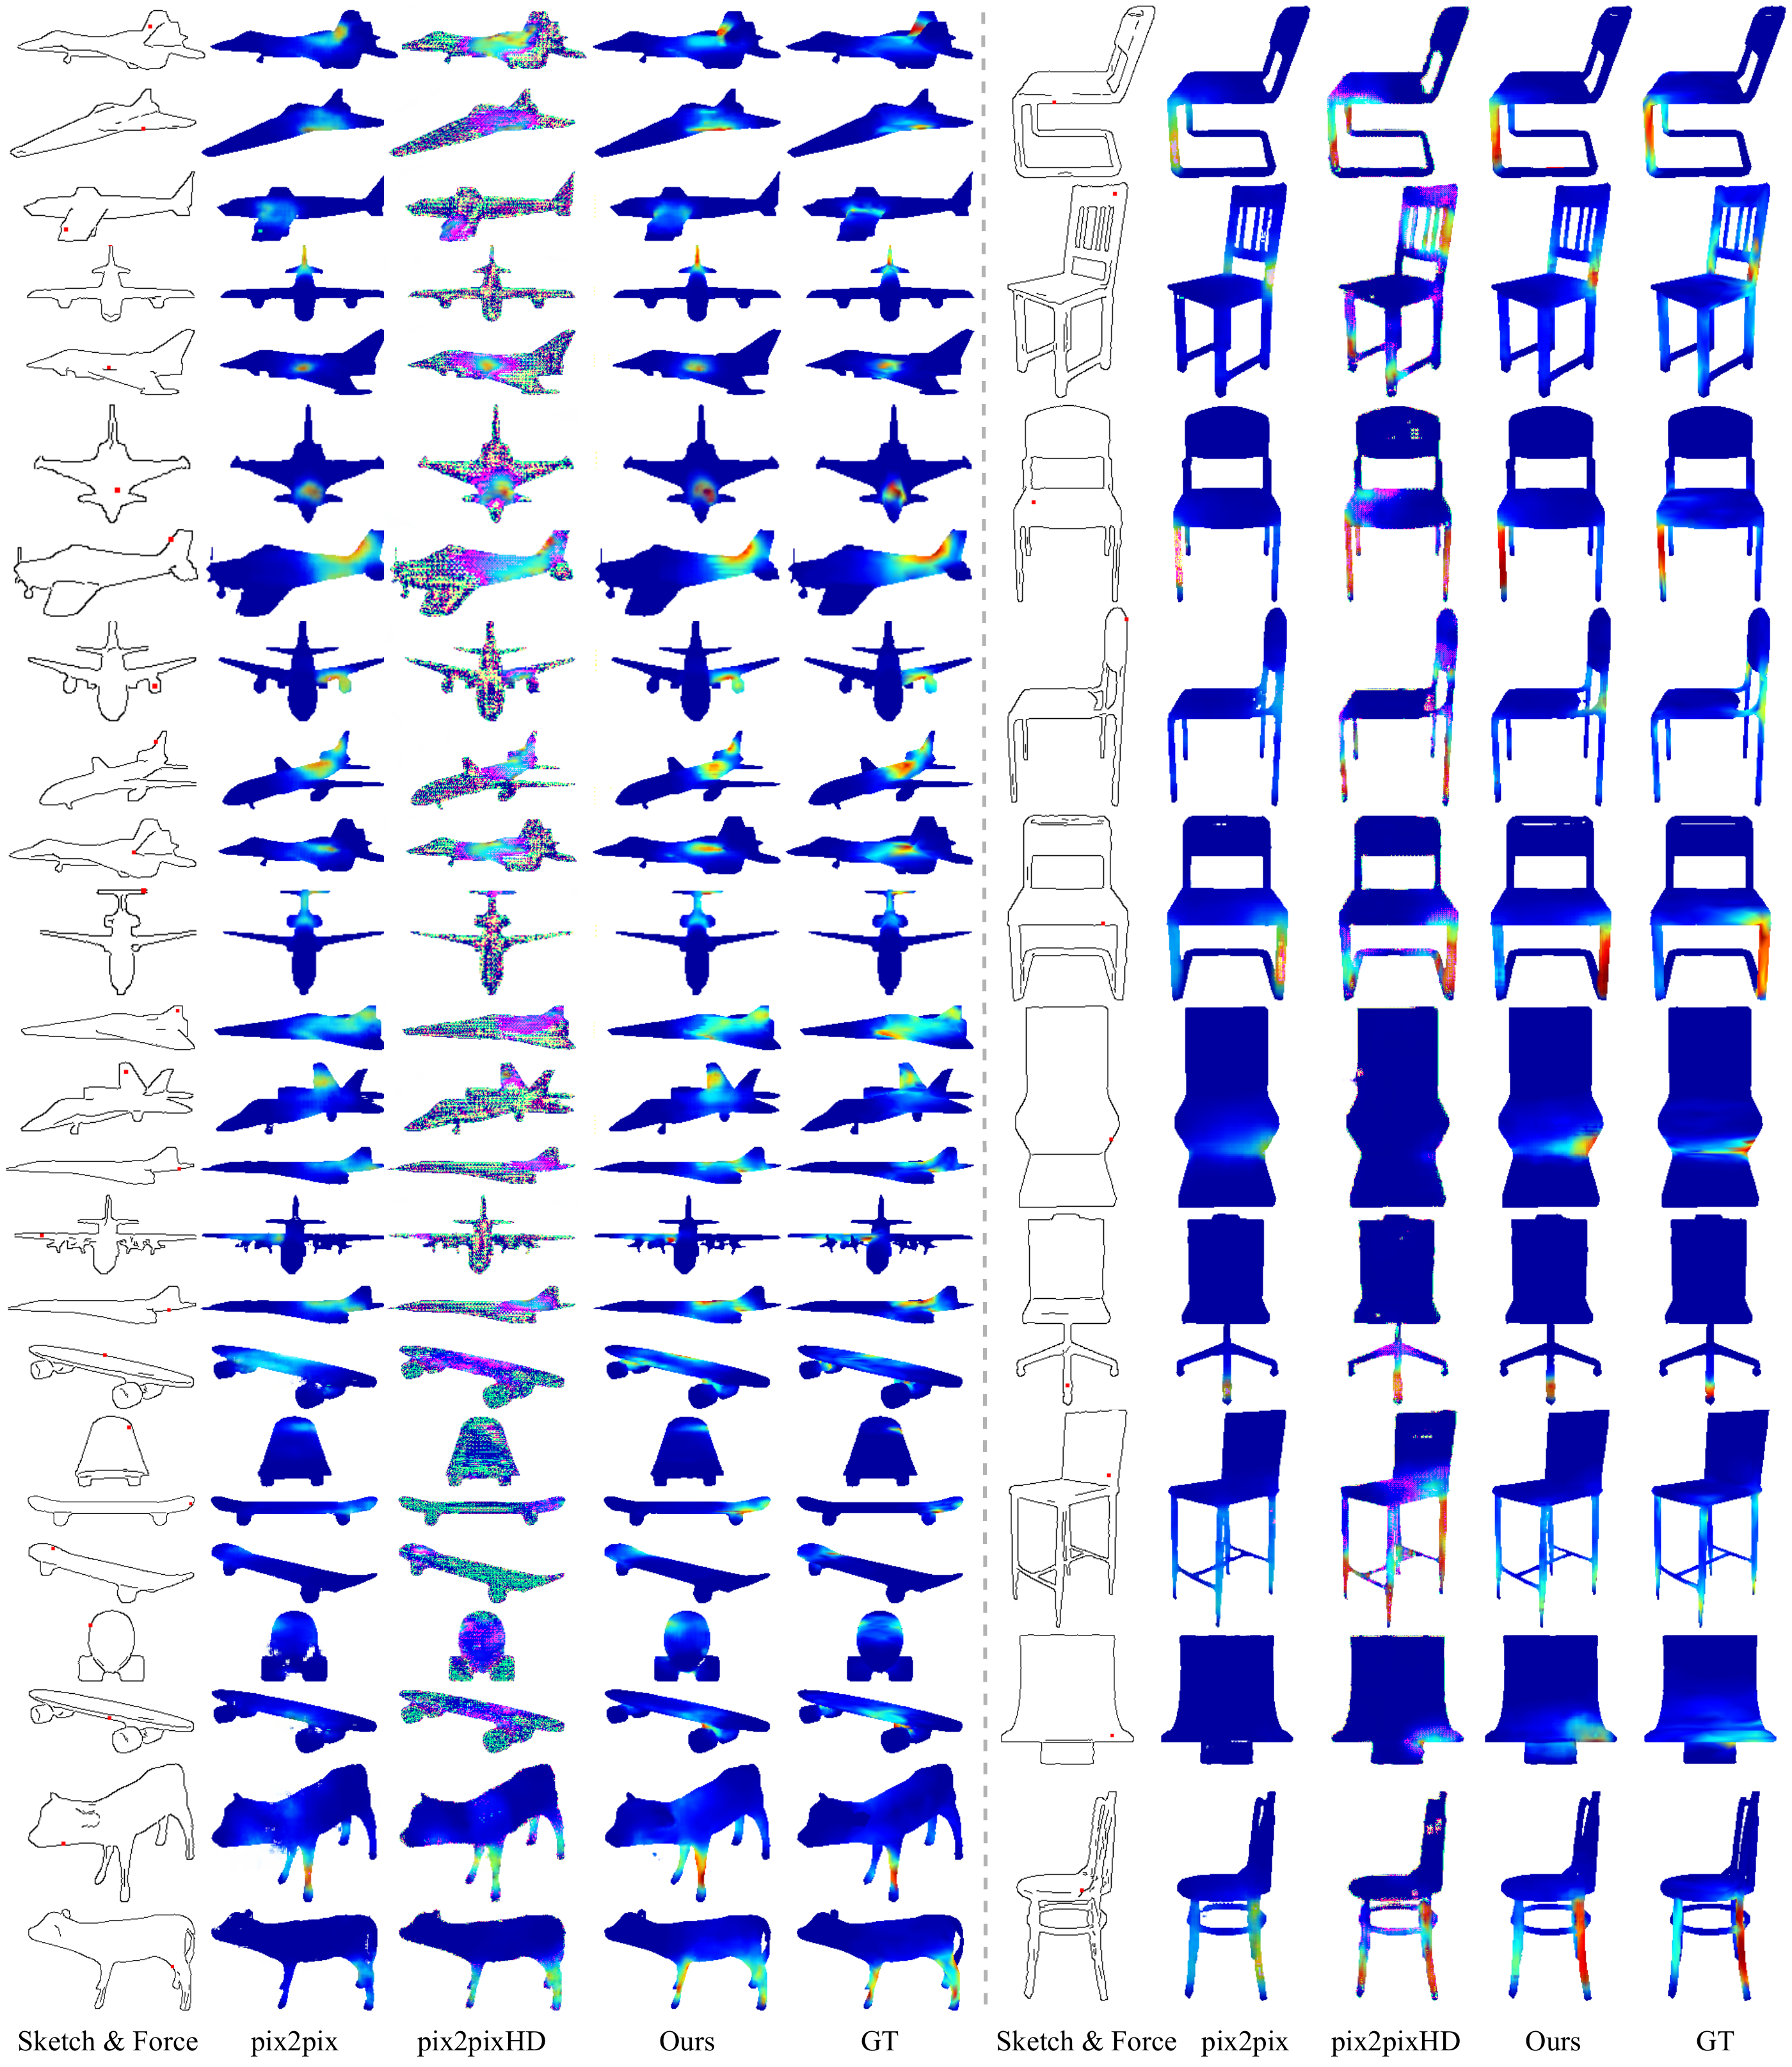}
    \caption{Qualitative comparison of {results generated by} %generation results of 
    different methods of pix2pix, pix2pixHD, our method, and ground truth.
    The leftmost column {shows} %s are 
    the input sketches and the external forces (plotted as red dots on sketches). 
    }
   
    \label{fig:qualtative_supple_A}
    }
\end{figure*}

\begin{figure*}[t]{
    \centering
    % \vspace{-5mm}
    \includegraphics[width=\linewidth]{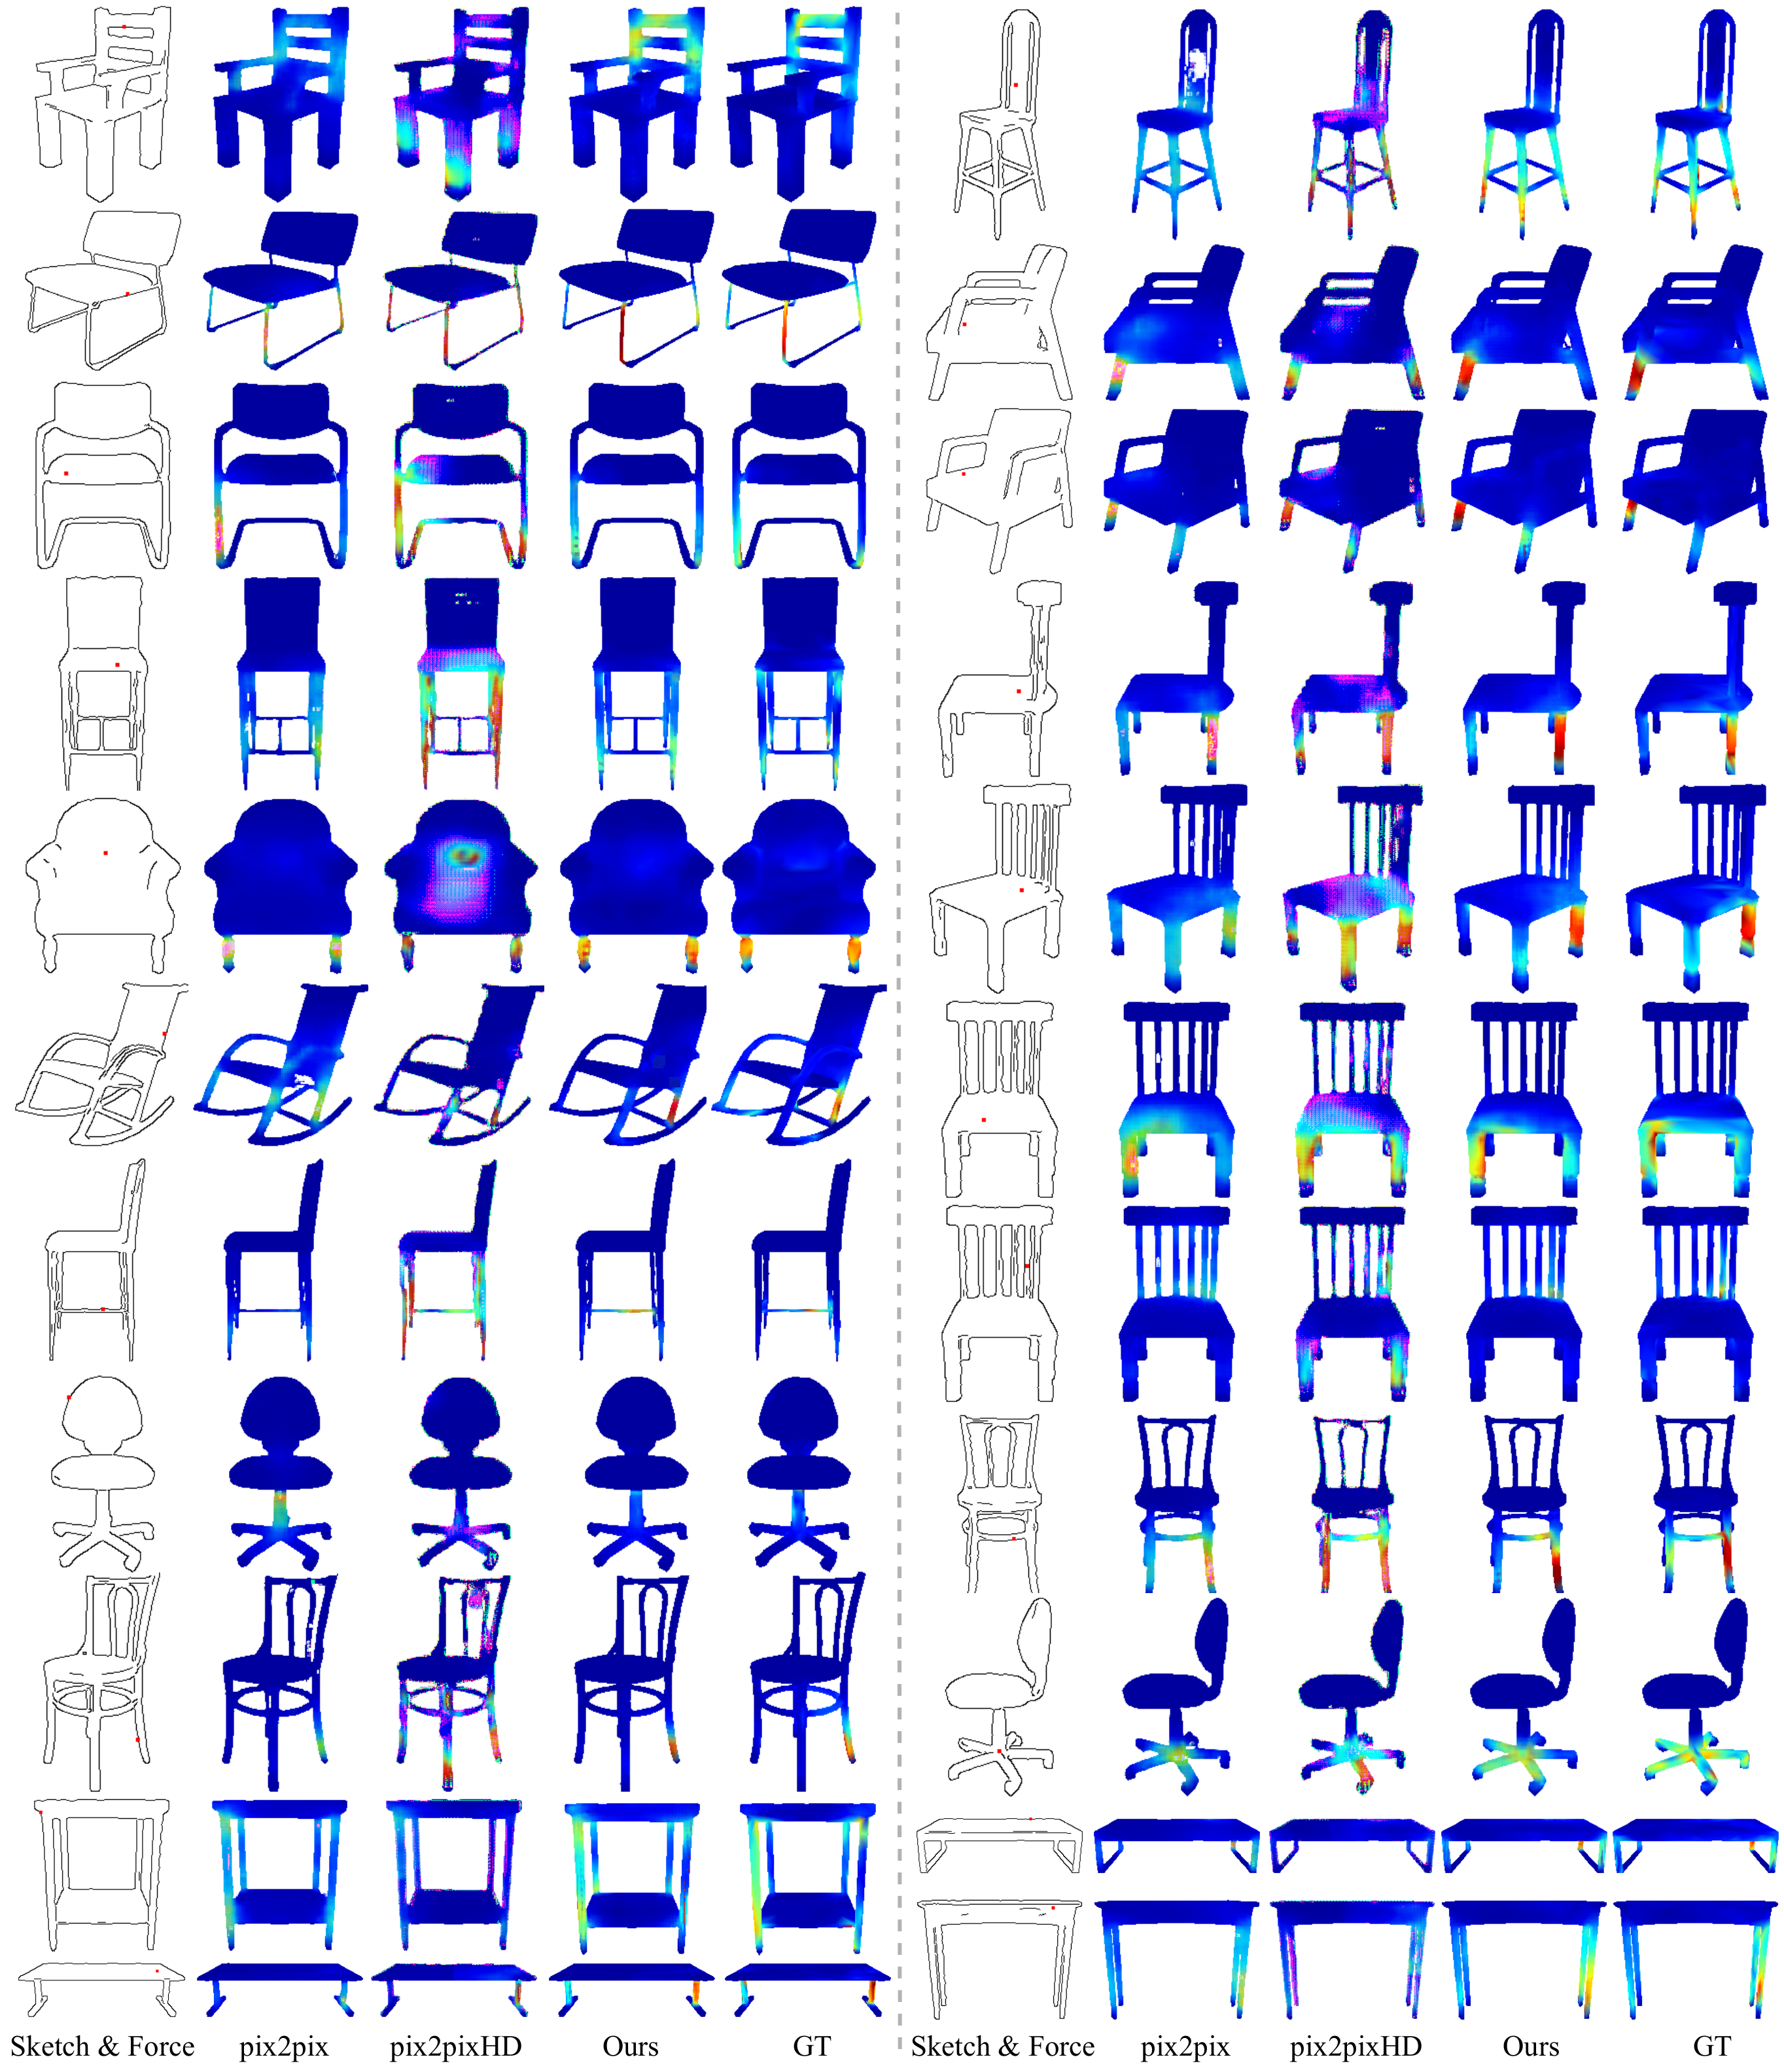}
    \caption{Qualitative comparison of {results generated by} %generation results of 
    different methods of pix2pix, pix2pixHD, our method, and ground truth.
    The leftmost column {shows} %s are 
    the input sketches and the external forces (plotted as red dots on sketches).  
    }
   
    \label{fig:qualtative_supple_B}
    }
\end{figure*}

\begin{figure*}[t]{
    \centering
    % \vspace{-5mm}
    \includegraphics[width=\linewidth]{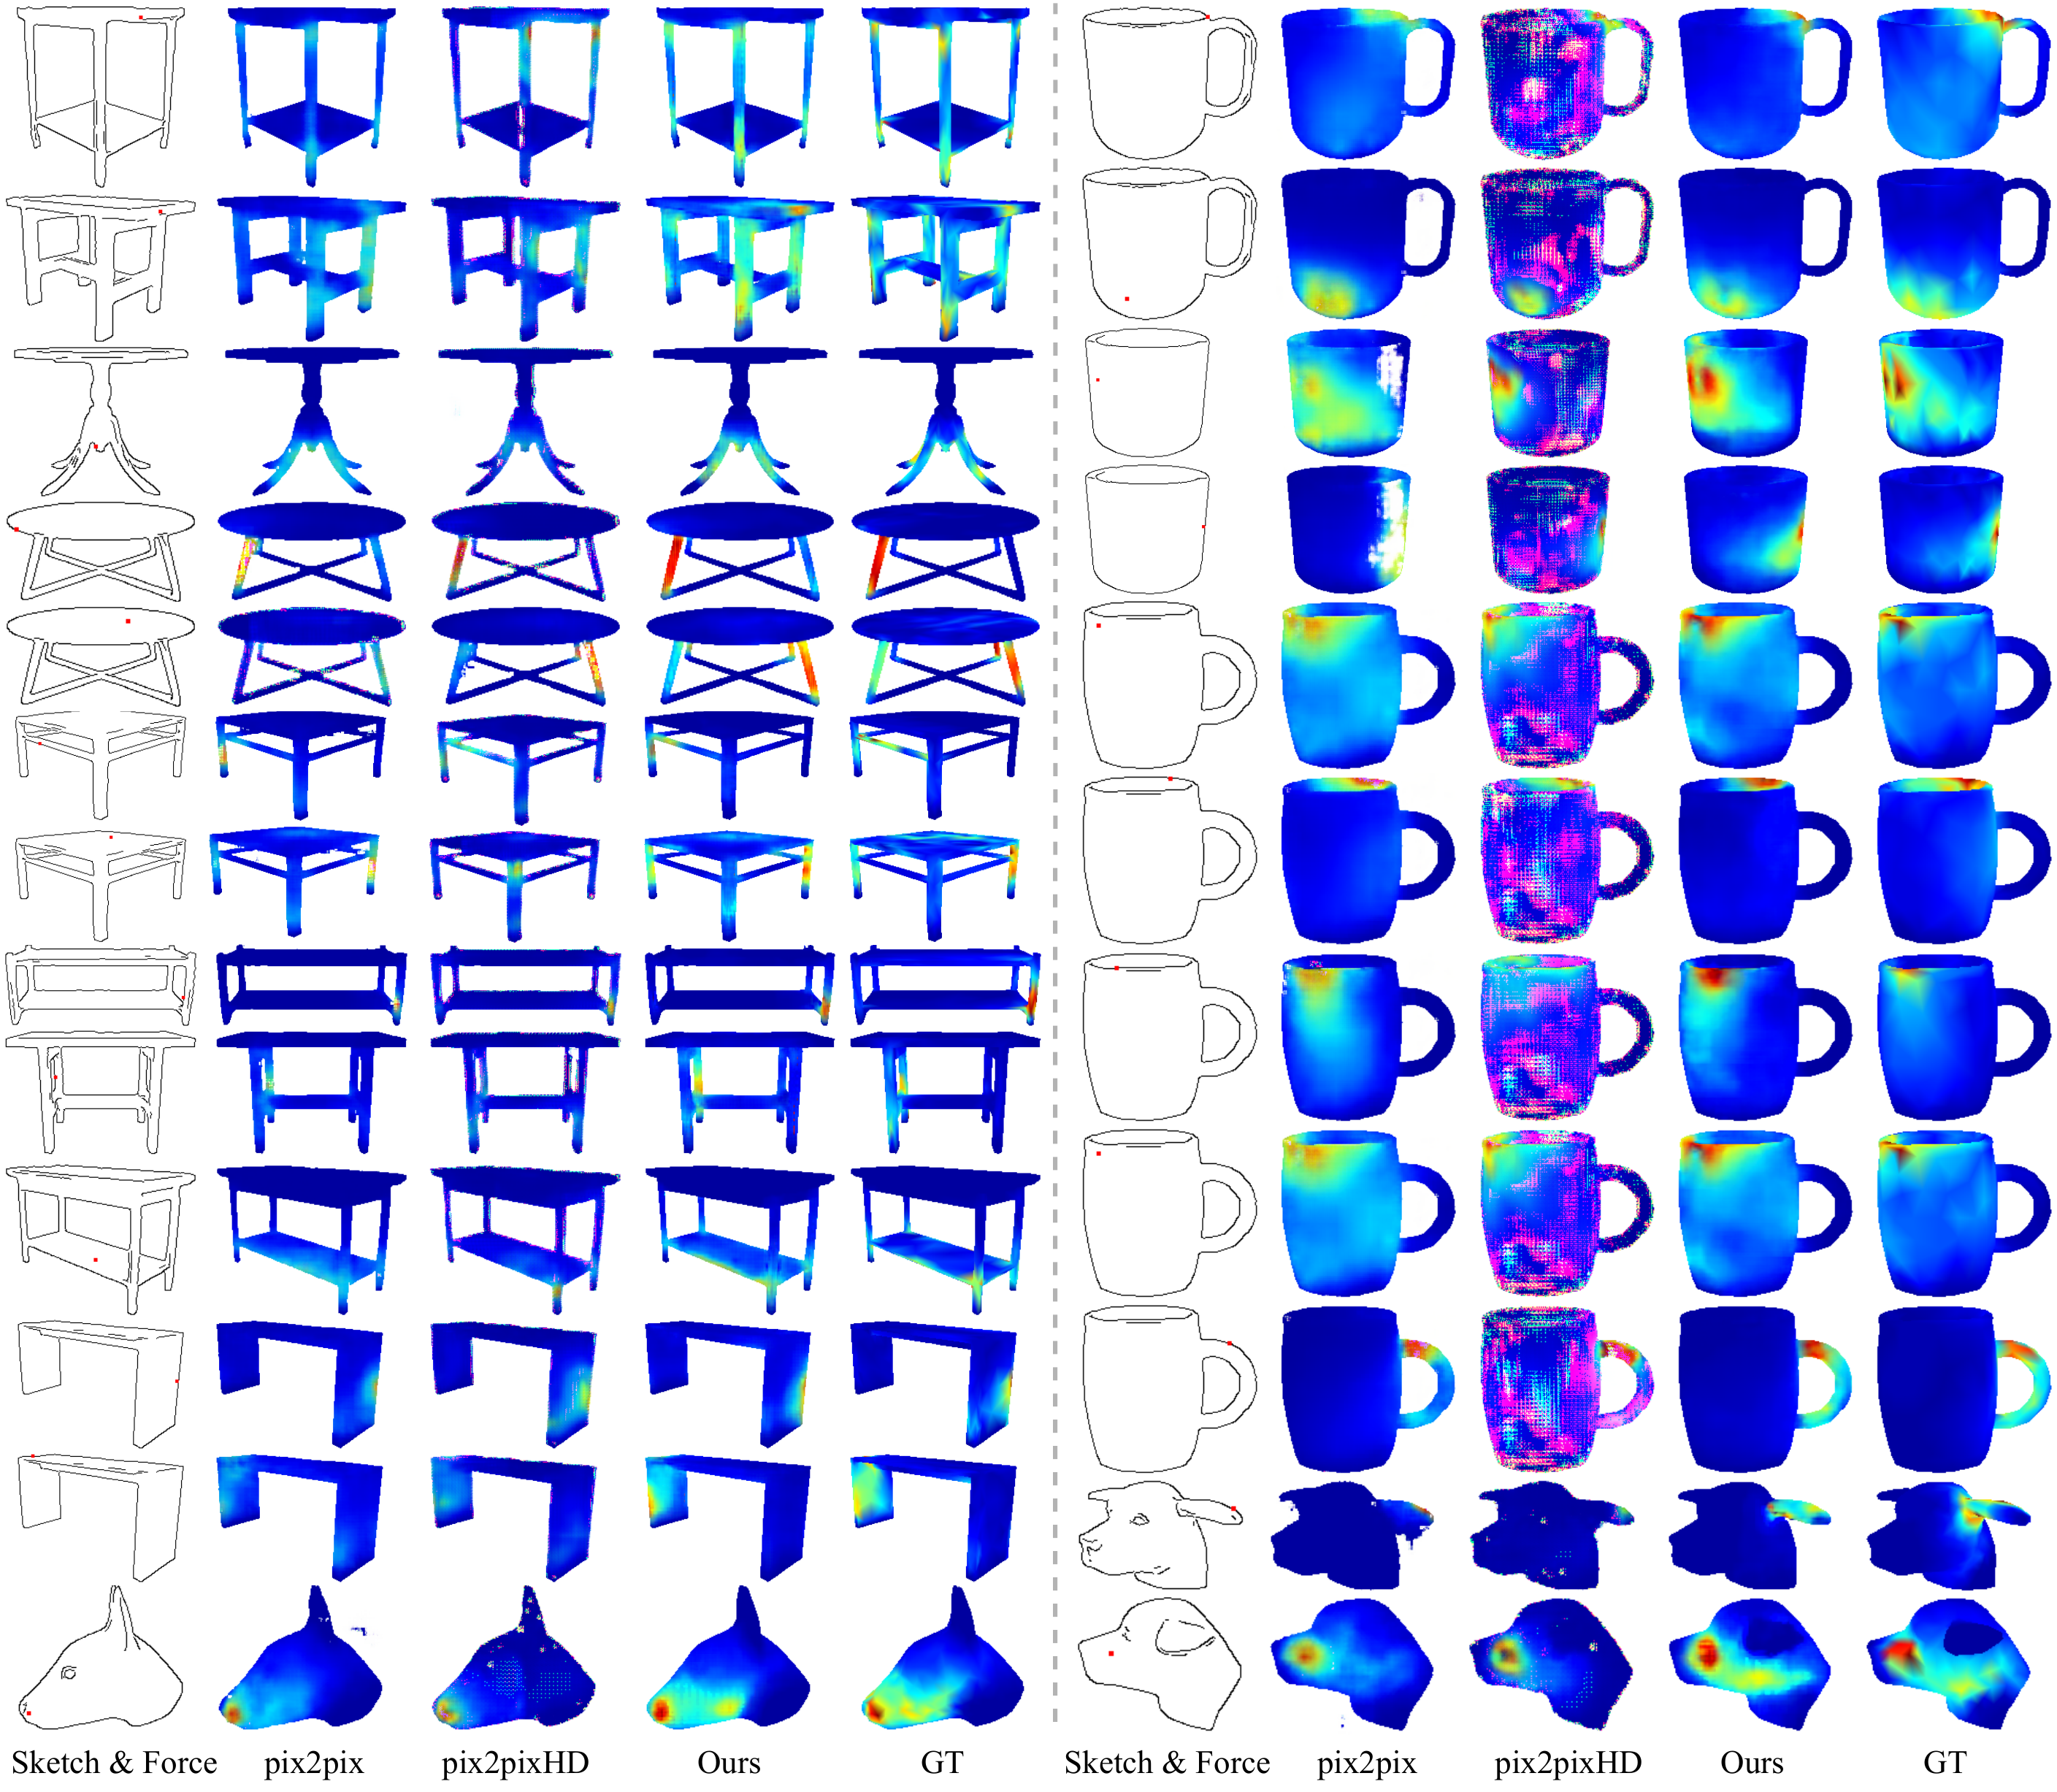}
    \caption{Qualitative comparison of {results generated by} 
    different methods of pix2pix, pix2pixHD, our method, and ground truth.
    The leftmost column {shows} %s are 
    the input sketches and the external forces (plotted as red dots on sketches).  
    }
   
    \label{fig:qualtative_supple_C}
    }
\end{figure*}
