# Supplementary material for: Sketch2Stress: Sketching with Structural Stress Awareness
Source: arXiv:2306.05911 source file (2023-12-11)
Supplement: Supplementary file 6 [file supplemental_abstract.tex]

\begin{abstract}

\end{abstract}
